# Supplementary material for: Method for finding the exact effective Hamiltonian of time driven quantum systems
Source: arXiv:1807.02550 ancillary file (2018-07-06)
Supplement: Supplementary file 1 [file supmat.pdf]

# Supplemental Material for
# "Method for finding the exact effective Hamiltonian of time driven quantum systems"

J. C. Sandoval-Santana,[1] V. G. Ibarra-Sierra,[1] J.L. Cardoso,[2] A. Kunold,[2] P. Roman-Taboada,[3] and G. G. Naumis[3]

[1]*Departamento de Física, Universidad Autónoma Metropolitana Iztapalapa, Av. San Rafael Atlixco 186, Col. Vicentina, 09340 Ciudad de México, México*
[2]*Departamento de Ciencias Básicas, Universidad Autónoma Metropolitana Azcapotzalco, Av. San Pablo 180, Col. Reynosa Tamaulipas, Ciudad de México, México*
[3]*Departamento de Sistemas Complejos, Instituto de Física, Universidad Nacional Autónoma de México, Apartado Postal 20-364 01000 Ciudad de México, México*

Here we show some of the details to obtain the effective Hamiltonians of the Paul trap, modulated optical lattice and the Kapitza pendulum.

## PAUL TRAP

### Deduction of the transformation parameters $\alpha_1(t), \alpha_2(t), \alpha_3(t)$

Let us first find the coefficients $\boldsymbol{u}$ of the transformed Hamiltonian. We thus substitute the structure constants into Eq. (12) to get

$$u_1 = \mathrm{e}^{4\alpha_2}\left(4a_3\alpha_1^2 - 4a_2\alpha_1 + a_1 - \dot{\alpha}_1\right), \tag{36}$$

$$u_2 = 2\mathrm{e}^{4\alpha_2}\alpha_3\left(4a_3\alpha_1^2 - 4a_2\alpha_1 + a_1 - \dot{\alpha}_1\right) - 2a_3\alpha_1 + a_2 - \dot{\alpha}_2, \tag{37}$$

$$u_3 = 4\mathrm{e}^{4\alpha_2}\alpha_3^2\left(4a_3\alpha_1^2 - 4a_2\alpha_1 + a_1 - \dot{\alpha}_1\right) + 4\alpha_3\left(-2a_3\alpha_1 + a_2 - \dot{\alpha}_2\right) + a_3\mathrm{e}^{-4\alpha_2} - \dot{\alpha}_3. \tag{38}$$

From the structure constants and Eq. (13) we build the $\nu$ matrix,

$$\nu = \begin{pmatrix} \mathrm{e}^{4\alpha_2(t)} & 0 & 0 \\ 2\mathrm{e}^{4\alpha_2(t)}\alpha_3(t) & 1 & 0 \\ 4\mathrm{e}^{4\alpha_2(t)}\alpha_3^2(t) & 4\alpha_3(t) & 1 \end{pmatrix}. \tag{39}$$

Using Eq. (14) and the coefficients $a_1 = m[\omega_1^2 + \omega_0^2\cos(\omega t)]/2$, $a_2 = 0$, $a_3 = 1/2m$, the time differential equations for the $\boldsymbol{\alpha}(t)$ parameters yield

$$\dot{\alpha}_1(t) = \frac{2}{m}\alpha_1^2(t) + \frac{m}{2}[\omega_1^2 + \omega_0^2\cos(\omega t)], \tag{40}$$

$$\dot{\alpha}_2(t) = -\frac{1}{m}\alpha_1(t), \tag{41}$$

$$\dot{\alpha}_3(t) = \frac{1}{2m}\mathrm{e}^{-4\alpha_2(t)}. \tag{42}$$

This system can be integrated to give Eqs. (23)-(25) in the main text

$$\alpha_1(t) = -\frac{m\omega^2}{8}\frac{d}{dt}\ln C(a,q,\omega t/2), \tag{23}$$

$$\alpha_2(t) = \frac{1}{2}\ln[C(a,q,\omega t/2)/C(a,q,0)], \tag{24}$$

$$\alpha_3(t) = \frac{C^2(a,q,0)}{2m}\int_0^t \frac{ds}{C^2(a,q,\omega s/2)}. \tag{25}$$

### Eigenvalue one eigenvector of $M_a^\top$

In the main text, the $\lambda$ differential equations are given in (26)-(28)

$$\partial_\lambda\alpha_1(\lambda,t) = \beta_1(t)\mathrm{e}^{-4\alpha_2(\lambda,t)}, \tag{26}$$

$$\partial_\lambda\alpha_2(\lambda,t) = \beta_2(t) - 2\beta_1(t)\alpha_3(\lambda,t), \tag{27}$$

$$\partial_\lambda\alpha_3(\lambda,t) = 4\beta_1(t)\alpha_3^2(\lambda,t) + \beta_3(t) - 4\beta_2(t)\alpha_3(\lambda,t). \tag{28}$$

The inverse relations of the form (18) that stem from them are rather difficult to obtain given the complexity of the resulting solutions for $\alpha_1(\lambda,t)$, $\alpha_2(\lambda,t)$ and $\alpha_3(\lambda,t)$. Therefore, we can calculate the eigenvalue one eigenvectors of $M_a^\top$ to reduce the number of free parameters. The transformation matrix $M_a^\top$, resulting from the definition (19) is the following,

$$M_a^\top = \mathrm{e}^{4\alpha_2(t)} \begin{pmatrix} 1 & -4\alpha_1(t) & 4\alpha_1^2(t) \\ 2\alpha_3(t) & \mathrm{e}^{-4\alpha_2(t)} - 8\alpha_1(t)\alpha_3(t) & 2\alpha_1(t)\left(4\alpha_1(t)\alpha_3(t) - \mathrm{e}^{-4\alpha_2(t)}\right) \\ 4\alpha_3^2(t) & 4\alpha_3(t)\left(\mathrm{e}^{-4\alpha_2(t)} - 4\alpha_1(t)\alpha_3(t)\right) & \left(\mathrm{e}^{-4\alpha_2(t)} - 4\alpha_1(t)\alpha_3(t)\right)^2 \end{pmatrix}. \tag{43}$$

This matrix only has one eigenvalue one eigenvector given by

$$\boldsymbol{\rho}(t) = \left(\frac{\alpha_1(t)}{\alpha_3(t)}, \frac{4\alpha_1(t)\alpha_3(t) - \mathrm{e}^{-4\alpha_2(t)} + 1}{4\alpha_3(t)}, 1\right). \tag{44}$$

Therefore, $\boldsymbol{\beta}(t)$ is parametrized by a single parameter $\gamma_1(t)$ (see main text)

$$\boldsymbol{\beta}(t) = \gamma_1(t)\left(\frac{\alpha_1(t)}{\alpha_3(t)}, \frac{4\alpha_1(t)\alpha_3(t) - \mathrm{e}^{-4\alpha_2(t)} + 1}{4\alpha_3(t)}, 1\right). \tag{29}$$

It suffices then to solve Eq. (28). By doing so we obtain

$$\alpha_3(t) = \frac{\beta_2(t) + \sqrt{\beta_1(t)\beta_3(t) - \beta_2^2(t)}\tan\left[2\gamma_1(t)\sqrt{\beta_1(t)\beta_3(t) - \beta_2^2(t)} - \tan^{-1}\left(\frac{\beta_2(t)}{\sqrt{\beta_1(t)\beta_3(t) - \beta_2^2(t)}}\right)\right]}{2\beta_1(t)}. \tag{45}$$

Clearing $\gamma_1(t)$ from the equation above

$$\gamma_1(t) = -\frac{2\alpha_3(t)}{16\alpha_1(t)\alpha_3(t) - \left(4\alpha_1(t)\alpha_3(t) - \mathrm{e}^{-4\alpha_2(t)} + 1\right)^2}\tan^{-1}\left[\frac{16\alpha_1(t)\alpha_3(t) - \left(4\alpha_1(t)\alpha_3(t) - \mathrm{e}^{-4\alpha_2(t)} + 1\right)^2}{4\alpha_1(t)\alpha_3(t) - 1 - \mathrm{e}^{-4\alpha_2(t)}}\right]. \tag{46}$$

Substituting the explicit form of $\gamma_1(t)$ in Eq. (29) we get the desired expression for $\boldsymbol{\beta}(t)$.

**Comparison with the known approximate solution.**

The effective Hamiltonian for a Paul trap was previously estimated in Ref. [1] for $\omega_1 = 0$ under the approximation $H_0 \ll V(t)$ giving

$$H_{\mathrm{e}} = \frac{p^2}{2m} + \frac{m\omega_0^4}{4\omega^2}x^2. \tag{47}$$

To compare our exact results with this approximation we introduce an expansion parameter $\delta$ into the Hamiltonian $H = \delta H_0 + V(t)$. To first order in $\delta$, the differential equations (40)-(42) take the form

$$\dot{\alpha}_1(t) = \dot{\alpha}_1^0(t) + \delta\dot{\alpha}_1^1(t) = \frac{1}{2}m\omega_0^2\cos(\omega t) + \delta\frac{2}{m}(\alpha_1^0(t))^2, \tag{48}$$

$$\dot{\alpha}_2(t) = \dot{\alpha}_2^0(t) + \delta\dot{\alpha}_2^1(t) = -\delta\frac{1}{m}\alpha_1^0(t), \tag{49}$$

$$\dot{\alpha}_3(t) = \dot{\alpha}_3^0(t) + \delta\dot{\alpha}_3^1(t) = \delta\frac{\mathrm{e}^{-4\alpha_2^0(t)}}{2m}. \tag{50}$$

Expanding to first order in $\delta$, their solutions are

$$\alpha_1(t) = \frac{m\omega_0^2}{2\omega}\sin(\omega t) + \delta\frac{m\omega_0^4}{2\omega^2}\left[\frac{t}{2} - \frac{\sin(\omega t)}{4\omega}\right], \tag{51}$$

$$\alpha_2(t) = \delta\frac{\omega_0^2}{\omega^2}\left[\cos(\omega t) - 1\right], \tag{52}$$

$$\alpha_3(t) = \delta\frac{t}{2m}. \tag{53}$$

Plugging the functions above to $\gamma_1(t)$ in Eq. (46), substituting into $\boldsymbol{\beta}(T)$ in Eq. (29) and expanding up to first order in $\delta$ we obtain

$$\beta_1(T) \approx \delta\alpha_{1,1}(T) = \delta\frac{m\omega_0^4 T}{4\omega^2}, \tag{54}$$
$$\beta_2(T) \approx \delta\alpha_{2,1}(T) = 0, \tag{55}$$
$$\beta_3(T) \approx \delta\alpha_{3,1}(T) = \delta\frac{T}{2m}. \tag{56}$$

These results clearly yield the effective Hamiltonian in Eq. (47) obtained in reference [1].

## MODULATED OPTICAL LATTICE.

To find the elements of a suitable Lie algebra for the modulated optical lattice Hamiltonian, we introduce $H_1 = iJ\sum_j(a_{j+1}^\dagger a_j - a_j^\dagger a_{j+1})$ to the preexisting $H_0 = J\sum_j(a_{j+1}^\dagger a_j + a_j^\dagger a_{j+1})$ and $V = \sum_j j a_j^\dagger a_j$ operators. It is clear that $h_1 = V$, $h_2 = H_1$ and $h_3 = H_0$ form a Lie algebra since $[h_1, h_2] = [V, H_1] = -iH_0 = -ih_3$, $[h_1, h_3] = [V, H_0] = iH_1 = ih_2$ and $[H_1, H_0] = [h_2, h_3] = 0$, where the corresponding non-vanishing structure constants are $c_{1,2,3} = -c_{2,1,3} = -1$ and $c_{1,3,2} = -c_{3,1,2} = 1$. From Eqs. (12) we calculate the coefficients of the transformed Hamiltonian $\boldsymbol{u}$

$$u_1 = a_1 - \dot{\alpha}_1(t), \tag{57}$$
$$u_2 = \alpha_3(t)\left(a_1 - \dot{\alpha}_1(t)\right) - a_3\sin(\alpha_1(t)) + a_2\cos(\alpha_1(t)) - \dot{\alpha}_2(t), \tag{58}$$
$$u_3 = a_2\sin(\alpha_1(t)) + a_3\cos(\alpha_1(t)) - \alpha_2(t)\left(a_1 - \dot{\alpha}_1(t)\right) - \dot{\alpha}_3(t), \tag{59}$$

where $a_1 = \omega\kappa\cos(\omega t)$, $a_2 = 0$ and $a_3 = 1$. Eq. (13) gives

$$\nu = \begin{pmatrix} 1 & 0 & 0 \\ \alpha_3(t) & 1 & 0 \\ -\alpha_2(t) & 0 & 1 \end{pmatrix}, \tag{60}$$

Plugging Eqs. (57)-(60) into (14) and replacing the Hamiltonian coefficients we obtain the following simplified system of ODE

$$\dot{\alpha}_1(t) = \omega\kappa\cos(\omega t), \tag{61}$$
$$\dot{\alpha}_2(t) = -\sin\left(\alpha_1(t)\right), \tag{62}$$
$$\dot{\alpha}_3(t) = \cos\left(\alpha_1(t)\right). \tag{63}$$

The solution to this ODE evaluated at $t = T$ is,

$$\alpha_1(T) = \alpha_2(T) = 0, \tag{64}$$
$$\alpha_3(T) = \frac{T}{2\pi}\int_0^{2\pi} d\tau\cos\left(\kappa\sin\tau\right) = TJ_0(\kappa), \tag{65}$$

where $J_0$ is the Bessel function of the first kind.

### Calculation via the solution of the $\lambda$ differential equations.

To get the relation between $\boldsymbol{\alpha}(t)$ and $\boldsymbol{\beta}(t)$ we first solve the ODE system arising from Eq. (16)

$$\partial_\lambda\alpha_1(\lambda, t) = \beta_1(t), \tag{66}$$
$$\partial_\lambda\alpha_2(\lambda, t) = \beta_2(t) - \beta_1(t)\alpha_3(\lambda, t), \tag{67}$$
$$\partial_\lambda\alpha_3(\lambda, t) = \beta_1(t)\alpha_2(\lambda, t) + \beta_3(t), \tag{68}$$

that yields

$$\alpha_1(\lambda, t) = \beta_1(t)\lambda, \tag{69}$$
$$\alpha_2(\lambda, t) = \frac{1}{\beta_1(t)}\left[\beta_2(t)\sin\left(\beta_1(t)\lambda\right) + \beta_3(t)\left(\cos\left(\beta_1(t)\lambda\right) - 1\right)\right], \tag{70}$$
$$\alpha_3(\lambda, t) = \frac{1}{\beta_1(t)}\left[\beta_3(t)\sin\left(\beta_1(t)\lambda\right) - \beta_2(t)\left(\cos\left(\beta_1(t)\lambda\right) - 1\right)\right]. \tag{71}$$

The $\boldsymbol{\beta}(t)$ parameters can be readily worked out by evaluating the previous expressions in $\lambda = 1$ and obtaining the inverse relation (18)

$$\beta_1(t) = \alpha_1(t), \tag{72}$$

$$\beta_2(t) = \frac{\alpha_1(t)}{2\,(1-\cos\alpha_1(t))}\left[\alpha_2(t)\sin\alpha_1(t) + \alpha_3(t)(1-\cos\alpha_1(t))\right], \tag{73}$$

$$\beta_3(t) = \frac{\alpha_1(t)}{2\,(1-\cos\alpha_1(t))}\left[\alpha_3(t)\sin\alpha_1(t) - \alpha_2(t)(1-\cos\alpha_1(t))\right]. \tag{74}$$

### Calculation via the eigenvalue one eigenvectors of $M_a^\top$.

These results can be reproduced by finding the eigenvalue one eigenvectors of $M_a^\top$, following the results in Eqs. (20) and (21). For the algebra regarding the optical lattice

$$M_a^\top = \begin{pmatrix} 1 & 0 & 0 \\ \alpha_3(t) & \cos(\alpha_1(t)) & -\sin(\alpha_1(t)) \\ -\alpha_2(t) & \sin(\alpha_1(t)) & \cos(\alpha_1(t)) \end{pmatrix}, \tag{75}$$

and the only eigenvector with eigenvalue equal to 1 is

$$\boldsymbol{\beta}(t) = \gamma_1(t)\left(2\frac{1-\cos\alpha_1(t)}{\alpha_3(t)\sin\alpha_1(t)+\alpha_2(t)\,(\cos\alpha_1(t)-1)}, \frac{\alpha_2(t)\sin\alpha_1(t)+\alpha_3(t)\,(1-\cos\alpha_1(t))}{\alpha_3(t)\sin\alpha_1(t)+\alpha_2(t)\,(1-\cos\alpha_1(t))}, 1\right). \tag{76}$$

The parameter $\gamma_1(t)$ can be determined just by using (66)

$$\gamma_1(t) = \alpha_1(t)\frac{\alpha_3(t)\sin\alpha_1(t)+\alpha_2(t)\,(\cos\alpha_1(t)-1)}{2\,(1-\cos\alpha_1(t))}, \tag{77}$$

and, finally, substituting this parameter into Eq. (76).

$$\beta_1(t) = \alpha_1(t), \tag{78}$$

$$\beta_2(t) = \frac{\alpha_1(t)}{2\,(1-\cos\alpha_1(t))}\left[\alpha_2(t)\sin\alpha_1(t) + \alpha_3(t)\,(1-\cos\alpha_1(t))\,\right], \tag{79}$$

$$\beta_3(t) = \frac{\alpha_1(t)}{2\,(1-\cos\alpha_1(t))}\left[\alpha_3(t)\sin\alpha_1(t) - \alpha_2(t)\,(1-\cos\alpha_1(t))\,\right]. \tag{80}$$

This method to find $\boldsymbol{\beta}(t)$ is considerably simpler than solving the system of differential equations and then working out the inverse relation. These results are identical to (72)-(74). Substituting (64)-(65) into the equations above we get

$$\beta_1(T) = \beta_2(T) = 0, \beta_3(T) = TJ_0(\kappa), \tag{81}$$

## KAPITZA PENDULUM

The coefficients $u$ from the transformed Hamiltonian can be calculated from Eq. (12) giving

$$u_1 = a_4 m^2\omega_0^2\alpha_3(t)^2 + a_4\alpha_2(t)^2 - a_3\alpha_2(t) + a_2\alpha_3(t) + a_1 - \dot\alpha_1(t) - \alpha_3(t)\dot\alpha_2(t), \tag{82}$$

$$u_2 = \cos\left(2m\omega_0\alpha_4(t)\right)\left[2a_4 m^2\omega_0^2\alpha_3(t) + a_2 - \dot\alpha_2(t)\right] - m\omega_0\left[-2a_4\alpha_2(t) + a_3 - \dot\alpha_3(t)\right]\sin\left(2\omega_0\alpha_4(t)\right), \tag{83}$$

$$u_3 = \frac{1}{m\omega_0}\sin\left(2m\omega_0\alpha_4(t)\right)\left[2a_4 m^2\omega_0^2\alpha_3(t) + a_2 - \dot\alpha_2(t)\right] + \left[-2a_4\alpha_2(t) + a_3 - \dot\alpha_3(t)\right]\cos\left(2m\omega_0\alpha_4(t)\right), \tag{84}$$

$$u_4 = a_4 - \dot\alpha_4(t). \tag{85}$$

From Eq. (13), the matrix obtained from the structure of the algebra yields,

$$\nu = \begin{pmatrix} 1 & \alpha_3(t) & 0 & 0 \\ 0 & \cos\left(2m\omega_0\alpha_4(t)\right) & -m\sin\left(2m\omega_0\alpha_4(t)\right)\omega_0 & 0 \\ 0 & \frac{1}{m\omega_0}\sin\left(2m\omega_0\alpha_4(t)\right) & \cos\left(2m\omega_0\alpha_4(t)\right) & 0 \\ 0 & 0 & 0 & 1 \end{pmatrix}. \tag{86}$$

Through Eq. (14), we get the following set of simplified coupled differential equations for the parameters,

$$\dot{\alpha}_1(t) = \frac{\alpha_2^2}{2m} - \frac{1}{2}m\omega_0^2\alpha_3^2(t), \quad (87)$$

$$\dot{\alpha}_2(t) = m\omega_0^2\alpha_3(t) + F\cos(\omega t), \quad (88)$$

$$\dot{\alpha}_3(t) = -\frac{\alpha_2(t)}{m}, \quad (89)$$

$$\dot{\alpha}_4(t) = \frac{1}{2m}. \quad (90)$$

The solution of this ODE system is given by

$$\alpha_1(t) = \frac{F^2 t\left(\omega^2-\omega_0^2\right)}{4m\left(\omega^2-\omega_0^2\right)^2} - \frac{F^2(\omega_0^2+\omega^2)\sin(2\omega t)}{8m\omega\left(\omega^2-\omega_0^2\right)^2} + \frac{F^2\omega_0\sin(\omega_0 t)[2\cos(\omega t)-\cos(\omega_0 t)]}{2m\left(\omega^2-\omega_0^2\right)^2}, \quad (91)$$

$$\alpha_2(t) = \frac{F[\omega\sin(\omega t)-\omega_0\sin(\omega_0 t)]}{\omega^2-\omega_0^2}, \quad (92)$$

$$\alpha_3(t) = \frac{F[\cos(\omega t)-\cos(\omega_0 t)]}{m(\omega^2-\omega_0^2)}, \quad (93)$$

$$\alpha_4(t) = \frac{t}{2m}. \quad (94)$$

To get the relation between $\boldsymbol{\alpha}(t)$ and $\boldsymbol{\beta}(t)$ we first solve the ODE system arising from Eq. (16)

$$\partial\lambda\alpha_1(\lambda,t) = \alpha_3(\lambda,t)\beta_3(t)m\omega_0\sin(2m\omega_0\alpha_4(\lambda,t)) + \alpha_3(\lambda,t)\beta_2(t)\cos(2m\omega_0\alpha_4(\lambda,t)) - \beta_1(t)\ , \quad (95)$$

$$\partial_\lambda\alpha_2(\lambda,t) = \beta_3(t)m\omega_0\sin(2m\omega_0\alpha_4(\lambda,t)) + \beta_2(t)\cos(2m\omega_0\alpha_4(\lambda,t))\ , \quad (96)$$

$$\partial_\lambda\alpha_3(\lambda,t) = \beta_3(t)\cos(2m\omega_0\alpha_4(\lambda,t)) - \frac{1}{m\omega_0}\beta_2(t)\sin(2m\omega_0\alpha_4(\lambda,t))\ , \quad (97)$$

$$\partial_\lambda\alpha_4(\lambda,t) = \beta_4(t). \quad (98)$$

The procedure to obtain the inverse relation (18) can be significantly simplified by computing the eigenvalue one eigenvectors of the transformation matrix $M_a^\top$. The transformation matrix $M_a^\top$, resulting from the definition Eq. (19) is the following,

$$M_a^\top = \begin{pmatrix} 1 & \alpha_3(t) & -\alpha_2(t) & m^2\omega_0^2\alpha_3^2(t)+\alpha_2^2(t) \\ 0 & \cos(2m\omega_0\alpha_4(t)) & -m\omega_0\sin(2m\omega_0\alpha_4(t)) & 2m\omega_0[\alpha_2(t)\sin(2m\omega_0\alpha_4(t))+m\omega_0\alpha_3(t)\cos(2m\omega_0\alpha_4(t))] \\ 0 & \frac{1}{m\omega_0}\sin(2m\omega_0\alpha_4(t)) & \cos(2m\omega_0\alpha_4(t)) & 2m\omega_0\alpha_3\sin(2m\omega_0\alpha_4(t)) - 2\alpha_2\cos(2m\omega_0\alpha_4(t)) \\ 0 & 0 & 0 & 1 \end{pmatrix}. \quad (99)$$

Two of such eigenvectors are found and consequently there are two unknown $\gamma_1(t), \gamma_2(t)$ parameters that give

$$\boldsymbol{\beta}(t) = \Big(\gamma_2(t), \gamma_1(t)m\omega_0[\alpha_2\cot(m\omega_0\alpha_4(t)) - m\omega_0\alpha_3(t)], \gamma_1(t)[m\omega_0\alpha_3(t)\cot(m\omega_0\alpha_4(t)) + \alpha_2(t)], \gamma_1(t)\Big). \quad (100)$$

From the ODE system (95)-(98), the expressions for these two parameters are found to be given by

$$\gamma_1(t) = \alpha_4(t), \quad (101)$$

$$\gamma_2(t) = \frac{\alpha_2^2(t)}{4}\left[\gamma_1(t)\csc^2(m\omega_0\gamma_1(t)) - \frac{\cot(m\omega_0\gamma_1(t))}{m\omega_0}\right] + \frac{m\omega_0\alpha_3^2(t)}{4}[m\omega_0\gamma_1(t)\csc^2(m\omega_0\gamma_1(t)) - \cot(m\omega_0\gamma_1(t))] + \frac{1}{2}\alpha_3(t)\alpha_2(t) + \alpha_1(t). \quad (102)$$

The four components of $\boldsymbol{\beta}(t)$ are calculated by substituting the explicit forms of $\gamma_1(t)$ and $\gamma_2(t)$ into Eq. (100).

[1] N. Goldman and J. Dalibard, Phys. Rev. X **4**, 031027 (2014).
