# Supplementary material for: Method for finding the exact effective Hamiltonian of time driven quantum systems
Source: arXiv:1807.02550 ancillary file (2018-07-06)
Supplement: Supplementary file 2 [file KapitzaPendulum.Mathematica.pdf]

# Kapitza Pendulum

---

## Modules

The following modules refer to the algebra

$$\mathcal{L}_n = \{h_1, \dots, h_n\},$$

that fulfils the commutation rule

$$[h_i, h_j] = i \hbar \sum_{k=1}^n c_{i,j,k} h_k,$$

characterized by the structure constants  $c_{i,k,j}$ .

## LieGetMa

**LieGetMa**[**c**, **J**, **vα**] generates the  $M$  transformations of the for  $M_k = e^{-Q_k}$  for  $k = 1, \dots,$

$n$  and  $M_{n+1} = M_1 \dots M_n$  is an  $n \times n$  matrix and  $M$  is an  $n \times n \times n$  tensor corresponding to the structure constants  $c$ .

- **c** :  $n \times n \times n$  tensor containing the structure constants,
- **J** :  $n \times n$  matrix,  $h' = Jh$  is a new representation of the  $\mathcal{L}_n$ ,
- **vα**: dimension  $n$  list  $v\alpha = \{\alpha_1, \alpha_2, \dots, \alpha_n\}$  containing the transformation parameters for the  $U_A$  transformation.

```

LieGetMa[c_, J_, v $\alpha$ _] := Module[{dim, k, Q, M},
  dim = Dimensions[c][[1]];
  k = Dimensions[J][[1]];
  M = Table[0, {k1, 1, k + 1}, {k2, 1, dim},
    {k3, 1, dim}];
  M[[k + 1]] = IdentityMatrix[k];
  Do[

    Q =
      Table[Sum[c[[k2, k3, k4]] J[[k1, k2]] v $\alpha$ [[k1]],
        {k2, 1, dim}], {k3, 1, dim}, {k4, 1, dim}];
    M[[k1]] = MatrixExp[-Q];
    M[[k + 1]] = M[[k + 1]].M[[k1]];
    , {k1, 1, k}];
  M
]

```

## LieGetNu

**LieGetNu[M,J]** generates the  $v$  matrix where  $v$  is an  $n \times n$  matrix.

- **M** :  $n \times n \times n$  tensor containing the transformation matrices,
- **J** :  $n \times n$  matrix,  $h' = Jh$  is a new representation of the  $\mathcal{L}_n$ .

```

LieGetNu[M_, J_] := Module[{dim, Mk, Ik, vt, vt1},
  dim = Dimensions[M[[1]]][[1]];
  Ik = Normal[SparseArray[{{1, 1} → 1}, dim]];
  vt1 = Ik.J;
  Do[
    Mk = M[[k1]];
    Ik = Normal[SparseArray[{{k1, k1} → 1}, dim]];
    vt = vt1.Mk + Ik.J;
    vt1 = vt;
    , {k1, 2, dim}];
  Transpose[vt]
]

```

## LieTrans

**LieTrans**[**M**, **J**, **va**, **va'**, **k**, **t**] transforms the coefficients  $h$  into  $va'$  under the  $k$ 'th transformation  $U_k$  corresponding to the  $M_k$  matrix. Under this transformation the original Floquet operator  $H - p_t = va^T h - p_t$  is transformed into  $H' - p_t = U_k (H - p_t) U_k = va^T M_k h - \alpha_k h_k - p_t = (va')^T h - p_t$  where  $va'$  is the new set of coefficients.

- **M** :  $n \times n \times n$  tensor containing the transformation matrices,
- **J** :  $n \times n$  matrix,  $h' = Jh$  is a new representation of the  $\mathcal{L}_n$ ,
- **va** : dimension  $n$  list  $va = \{a_1, a_2, \dots, a_n\}$  containing the coefficients of the original Floquet operator,

- **$\mathbf{v}\alpha$**  : dimension  $n$  list  $\mathbf{v}\alpha = \{\alpha_1, \alpha_2, \dots, \alpha_n\}$  containing the transformation parameters for the  $U_A$  transformation,
- **$\mathbf{k}$**  : integer that tags the number of transformation to be used,
- **$\mathbf{t}$**  : time parameter.

```
LieTrans[M_, J_, va_, vα_, k_, t_] :=  
  va.M[[k]] - D[vα[[k]], t] J[[k]]
```

## LieGetu

**LieGetu[M, J, va, vα, t]** transforms the original coefficients  $\mathbf{v}\alpha$  into  $\mathbf{u}$  under the complete transformation  $U_A$  corresponding to  $M_\alpha = M_1 M_2 \dots M_n$ . Under this transformation the original Floquet operator  $H - p_t = \mathbf{v}\alpha \cdot \mathbf{h} - p_t$  is transformed into  $H' - p_t = U_A (H - p_t) U_A = \mathbf{v}\alpha^T M_\alpha \mathbf{h} - \dot{\alpha}^T \mathbf{v}^T \mathbf{h}_k - p_t = \mathbf{u}^T \mathbf{h} - p_t$ .

- **$\mathbf{M}$**  : is an  $n \times n \times n$  tensor containing the transformation matrices,
- **$\mathbf{J}$**  :  $n \times n$  matrix,  $\mathbf{h}' = \mathbf{J}\mathbf{h}$  is a new representation of the  $\mathcal{L}_n$ ,
- **$\mathbf{v}\alpha$**  : dimension  $n$  list  $\mathbf{v}\alpha = \{\alpha_1, \alpha_2, \dots, \alpha_n\}$  containing the coefficients of the original Floquet operator,
- **$\mathbf{v}\alpha$**  : dimension  $n$  list containing the transformation parameters for the  $U_A$  transformation. The  $\alpha$  parameters must be functions of the time parameter  $t$ .
- **$\mathbf{t}$**  : time parameter.

```

LieGetu[M_, J_, va_, v $\alpha$ _, t_] := Module[{k, vu, vw},
  k = Dimensions[v $\alpha$ ][[1]];
  vu = va;
  Do[
    vw = LieTrans[M, J, vu, v $\alpha$ , k1, t];
    vu = vw;
    , {k1, 1, k}];
  vu
]

```

## LieGetDifEqLambda

**LieGetDifEqLambda[J,vi,v $\alpha$ ,v $\beta$ , $\lambda$ ,ci]** calculates a list containing the differential equations with respect to the auxiliary parameter  $\lambda$  that connects the  $\alpha$  and  $\beta$  parameters.

- **J** :  $n \times n$  matrix,  $h' = J.h$  is a new representation of the  $\mathcal{L}_n$ ,
- **vi** : inverse of the  $n \times n$  matrix  $v$  calculated with LieGetNu[M,J],
- **v $\alpha$**  : dimension  $n$  list  $v\alpha = \{\alpha_1, \alpha_2, \dots, \alpha_n\}$  containing the transformation parameters for the  $U_A$ . The  $\alpha$  parameters must be functions of the auxiliary parameter  $\lambda$ ,
- **v $\beta$**  : dimension  $n$  list  $v\beta = \{\beta_1, \beta_2, \dots, \beta_n\}$  containing the transformation parameters for the  $U_B$ . The  $\beta$  parameters are NOT functions of the auxiliary parameter  $\lambda$ ,
- **$\lambda$**  : is the auxiliary parameter that helps relate the  $\alpha$  and  $\beta$  transformation parameters.

**ci** : is a Boolean variable. If  $ci == \text{True}$ ,  
the initial conditions  $\alpha_1[0] == 0$ ,  $\alpha_2[0] == 0$ , ...,  
 $\alpha_n[0] == 0$  is appended to the list of differential equations. If on  $ci ==$   
False then the output is just the list of differential equations,

- **$\lambda$**  : is the auxiliary parameter that helps relate the  $\alpha$  and  $\beta$  transformation parameters.

```
LieGetDifEqLambda[J_, v i_, v  $\alpha$ _, v  $\beta$ _,  $\lambda$ _, ci_] :=
Module[{dim, v},
  dim = Dimensions[v  $\alpha$ ][[1]];
  v = v i. v  $\beta$ ;
  If[ci == True,
    Join[Table[D[v  $\alpha$ [[k1]],  $\lambda$ ] == v[[k1]], {k1, 1, dim}],
      Table[(v  $\alpha$ [[k1]] /.  $\lambda \rightarrow 0$ ) == 0, {k1, 1, dim}]],
    Table[D[v  $\alpha$ [[k1]],  $\lambda$ ] == v[[k1]], {k1, 1, dim}]
  ]
]
```

---

## Main Program

### Definition of the structure constants $c_{i,j,k}$

The elements of this algebra are given by the operators  $h_1 = 1$ ,  
 $h_2 = x$ ,  $h_3 = p$ ,  $h_4 = m \omega_0^2 x^2 + p^2$ . The following lines define the  
algebra dimension and the structure constants.

```

n = 4;
d = Table[0, {k1, 1, n}, {k2, 1, n}, {k3, 1, n}];
d[[2, 3, 1]] = 1;
d[[3, 2, 1]] = -1;
d[[4, 2, 3]] = -2;
d[[2, 4, 3]] = 2;
d[[4, 3, 2]] = 2 m2 ω02;
d[[3, 4, 2]] = -2 m2 ω02;

R = IdentityMatrix[n];
Ri = Inverse[R];
c =
  Table[Sum[R[[k1, m1]] R[[k2, m2]] Ri[[m3, k3]]
    d[[m1, m2, m3]], {m1, 1, n}, {m2, 1, n},
    {m3, 1, n}], {k1, 1, n}, {k2, 1, n}, {k3, 1, n}];

```

Since  $J=\mathcal{I}$ , the structure of the algebra elements is preserved.

```
J = IdentityMatrix[n];
```

## Derivation of the time differential equations for $\alpha_i(t)$

We calculate  $\mathcal{U}$  using Eq. (12). Notice that in this case  $v\alpha = \{\alpha_1(t), \dots, \alpha_n(t)\}$  is a function of time.

```

vα = Table[Subscript[α, k1][t], {k1, 1, n}];
va = Table[Subscript[a, k1], {k1, 1, n}];
Ma = LieGetMa[c, J, vα];
vu = LieGetu[Ma, J, va, vα, t];
MatrixForm[Simplify[ExpToTrig[vu]]]

```

$$\begin{pmatrix} a_1 - a_3 \alpha_2[t] + a_4 \alpha_2[t]^2 + a_2 \alpha_3[t] + m^2 a_4 \omega_0^2 \alpha_3[t]^2 \cdot \\ \cos[2 m \omega_0 \alpha_4[t]] (a_2 + 2 m^2 a_4 \omega_0^2 \alpha_3[t] - \alpha_2'[t]) - m \sin[2 m \omega_0 c \\ \frac{\sin[2 m \omega_0 \alpha_4[t]] (a_2 + 2 m^2 a_4 \omega_0^2 \alpha_3[t] - \alpha_2'[t])}{m \omega_0} + \cos[2 m \omega_0 \alpha_4[t]] \\ a_4 - \alpha_4'[t] \end{pmatrix}$$

Compare these results with the ones in Eqs. (82)-(85).

The simplified differential equations for  $\alpha_i(t)$  are obtained from Eq. (14)

```

v = LieGetNu[Ma, J];
vi = Inverse[v];
ε = Simplify[vi.vu];
MatrixForm[ε]

```

$$\begin{pmatrix} a_1 - a_3 \alpha_2[t] + a_4 \alpha_2[t]^2 - m^2 a_4 \omega_0^2 \alpha_3[t]^2 - \alpha_1'[t] \\ a_2 + 2 m^2 a_4 \omega_0^2 \alpha_3[t] - \alpha_2'[t] \\ a_3 - 2 a_4 \alpha_2[t] - \alpha_3'[t] \\ a_4 - \alpha_4'[t] \end{pmatrix}$$

Compare these results with the ones in Eqs. (87)-(90).

## Relation between $\alpha(t)$ and $\beta(t)$ via the solution of the $\lambda$ differential equations

Using Eq. (16) we workout the  $\lambda$  differential equations for the  $\alpha_i(\lambda, t)$  parameters. Note that in this case  $v\alpha = \{\alpha_1(\lambda), \dots, \alpha_n(\lambda)\}$  is a function of  $\lambda$  therefore,  $M_a$  and  $v$  have to be recalculated. In

**LieGetDifEqLamda** the condition **ci** is set to **True** in order to



include the initial conditions.

```

vα = Table[Subscript[α, k1][λ], {k1, 1, n}];
Ma = LieGetMa[c, J, vα];
v = LieGetNu[Ma, J];
vi = Inverse[v];
vβ = Table[Subscript[β, k1], {k1, 1, n}];
difeqsλ =
  Simplify[
    ExpToTrig[LieGetDifEqLambda[J, vi, vα, vβ, λ,
      True]]];
MatrixForm[difeqsλ]

```

$$\left( \begin{array}{l}
 (\cos[2 m \omega_0 \alpha_4[\lambda]] \beta_2 + m \sin[2 m \omega_0 \alpha_4[\lambda]] \beta_3 \omega_0) \alpha_3[\lambda] + \alpha_1'[\lambda] \\
 \cos[2 m \omega_0 \alpha_4[\lambda]] \beta_2 + m \sin[2 m \omega_0 \alpha_4[\lambda]] \beta_3 \omega_0 = \alpha_2'[\lambda] \\
 \cos[2 m \omega_0 \alpha_4[\lambda]] \beta_3 = \frac{\sin[2 m \omega_0 \alpha_4[\lambda]] \beta_2}{m \omega_0} + \alpha_3'[\lambda] \\
 \beta_4 = \alpha_4'[\lambda] \\
 \alpha_1[0] == 0 \\
 \alpha_2[0] == 0 \\
 \alpha_3[0] == 0 \\
 \alpha_4[0] == 0
 \end{array} \right)$$

Compare these results with Eqs. (95)-(98).

These equations are simple enough that we can attempt to solve them with **DSolve**.

`sol = Simplify[DSolve[difeqsλ, va, λ][[1]]]`

$$\left\{ \alpha_4[\lambda] \rightarrow \lambda \beta_4, \alpha_2[\lambda] \rightarrow \frac{\sin[m \lambda \beta_4 \omega_0] (\cos[m \lambda \beta_4 \omega_0] \beta_2 + m \sin[m \lambda \beta_4 \omega_0] \beta_3 \omega_0)}{m \beta_4 \omega_0}, \right.$$

$$\alpha_3[\lambda] \rightarrow \frac{-2 \sin[m \lambda \beta_4 \omega_0]^2 \beta_2 + m \sin[2 m \lambda \beta_4 \omega_0] \beta_3 \omega_0}{2 m^2 \beta_4 \omega_0^2},$$

$$\alpha_1[\lambda] \rightarrow \frac{1}{16 m^3 \beta_4^2 \omega_0^3} \left( -8 m \cos[2 m \lambda \beta_4 \omega_0] \sin[m \lambda \beta_4 \omega_0]^2 \beta_2 \beta_3 \omega_0 - \beta_2^2 \right.$$

$$\left. (-4 \sin[2 m \lambda \beta_4 \omega_0] + \sin[4 m \lambda \beta_4 \omega_0] + 4 m \lambda \beta_4 \omega_0) + m^2 \omega_0^2 (16 m \lambda \beta_1 \beta_4^2 \omega_0 + \beta_3^2 (\sin[4 m \lambda \beta_4 \omega_0] - 4 m \lambda \beta_4 \omega_0)) \right)$$

Setting  $\lambda=1$  we can obtain a relation between  $\alpha(t)$  and  $\beta(t)$  of the form (17).

`va1 = Table[Subscript[α, k1], {k1, 1, n}];`  
`eqs = Table[va1[[k1]] == ((va[[k1]] /. sol) /. {λ → 1}),`  
`{k1, 1, n}]`

$$\left\{ \alpha_1 == \frac{1}{16 m^3 \beta_4^2 \omega_0^3} \left( -8 m \cos[2 m \beta_4 \omega_0] \sin[m \beta_4 \omega_0]^2 \beta_2 \beta_3 \omega_0 - \right. \right.$$

$$\left. \beta_2^2 (-4 \sin[2 m \beta_4 \omega_0] + \sin[4 m \beta_4 \omega_0] + 4 m \beta_4 \omega_0) + m^2 \omega_0^2 (16 m \beta_1 \beta_4^2 \omega_0 + \beta_3^2 (\sin[4 m \beta_4 \omega_0] - 4 m \beta_4 \omega_0)) \right),$$

$$\alpha_2 == \frac{\sin[m \beta_4 \omega_0] (\cos[m \beta_4 \omega_0] \beta_2 + m \sin[m \beta_4 \omega_0] \beta_3 \omega_0)}{m \beta_4 \omega_0},$$

$$\alpha_3 == \frac{-2 \sin[m \beta_4 \omega_0]^2 \beta_2 + m \sin[2 m \beta_4 \omega_0] \beta_3 \omega_0}{2 m^2 \beta_4 \omega_0^2},$$

$$\alpha_4 == \beta_4 \}$$

## Relation between $\alpha(t)$ and $\beta(t)$ via the eigenvalue one eigenvectors of $M_a^T$

Working out the inverse relation between  $\alpha$  and  $\beta$  might be difficult in this case given the complexity of the previous equations.

Therefore, it is convenient to obtain a relation between  $\alpha(t)$  and  $\beta(t)$  by obtaining the eigenvalue one eigenvectors of  $M_a^T$ . There are two eigenvalue one eigenvectors.

```

vα = Table[Subscript[α, k1], {k1, 1, n}];
Ma = LieGetMa[c, J, vα];
Mat = Transpose[Ma[[n + 1]]];
eval = Simplify[Eigenvalues[Mat]];
evec = Simplify[Eigenvectors[Mat]];
eval[[2]]
ρ1 = Simplify[ExpToTrig[evec[[2]]]]
eval[[3]]
ρ2 = Simplify[evec[[3]]]
vβ = γ1 ρ1 + γ2 ρ2

```

1

$$\{0, -m \omega_0 (-\cot[m \alpha_4 \omega_0] \alpha_2 + m \alpha_3 \omega_0), \\ \alpha_2 + m \cot[m \alpha_4 \omega_0] \alpha_3 \omega_0, 1\}$$

1

$$\{1, 0, 0, 0\}$$

$$\{\gamma_2, -m \gamma_1 \omega_0 (-\cot[m \alpha_4 \omega_0] \alpha_2 + m \alpha_3 \omega_0), \\ \gamma_1 (\alpha_2 + m \cot[m \alpha_4 \omega_0] \alpha_3 \omega_0), \gamma_1\}$$

Compare this last result with the one in Eq. (100).
