# Supplementary material for: Method for finding the exact effective Hamiltonian of time driven quantum systems
Source: arXiv:1807.02550 ancillary file (2018-07-06)
Supplement: Supplementary file 4 [file PaulTrap.Mathematica.pdf]

# Paul Trap

---

## Modules

The following modules refer to the algebra

$$\mathcal{L}_n = \{h_1, \dots, h_n\},$$

that fulfils the commutation rule

$$[h_i, h_j] = i \hbar \sum_{k=1}^n c_{i,j,k} h_k,$$

characterized by the structure constants  $c_{i,k,j}$ .

## LieGetMa

**LieGetMa**[**c**, **J**, **vα**] generates the  $M$  transformations of the for  $M_k = e^{-Q_k}$  for  $k = 1, \dots,$

$n$  and  $M_{n+1} = M_1 \dots M_n$  is an  $n \times n$  matrix and  $M$  is an  $n \times n \times n$  tensor corresponding to the structure constants  $c$ .

- **c** :  $n \times n \times n$  tensor containing the structure constants,
- **J** :  $n \times n$  matrix,  $h' = Jh$  is a new representation of the  $\mathcal{L}_n$ ,
- **vα**: dimension  $n$  list  $v\alpha = \{\alpha_1, \alpha_2, \dots, \alpha_n\}$  containing the transformation parameters for the  $U_A$  transformation.

```

In[1]:= LieGetMa[c_, J_, v $\alpha$ _] := Module[{dim, k, Q, M},
  dim = Dimensions[c][[1]];
  k = Dimensions[J][[1]];
  M = Table[0, {k1, 1, k + 1}, {k2, 1, dim},
    {k3, 1, dim}];
  M[[k + 1]] = IdentityMatrix[k];
  Do[

    Q =
      Table[Sum[c[[k2, k3, k4]] J[[k1, k2]] v $\alpha$ [[k1]],
        {k2, 1, dim}], {k3, 1, dim}, {k4, 1, dim}];
    M[[k1]] = MatrixExp[-Q];
    M[[k + 1]] = M[[k + 1]].M[[k1]];
    , {k1, 1, k}];
  M
]

```

## LieGetNu

**LieGetNu[M,J]** generates the  $v$  matrix where  $v$  is an  $n \times n$  matrix.

- **M** :  $n \times n \times n$  tensor containing the transformation matrices,
- **J** :  $n \times n$  matrix,  $h' = Jh$  is a new representation of the  $\mathcal{L}_n$ .

```

In[2]:= LieGetNu[M_, J_] := Module[{dim, Mk, Ik, vt, vt1},
  dim = Dimensions[M[[1]]][[1]];
  Ik = Normal[SparseArray[{{1, 1} → 1}, dim]];
  vt1 = Ik.J;
  Do[
    Mk = M[[k1]];
    Ik = Normal[SparseArray[{{k1, k1} → 1}, dim]];
    vt = vt1.Mk + Ik.J;
    vt1 = vt;
    , {k1, 2, dim}];
  Transpose[vt]
]

```

## LieTrans

**LieTrans**[**M**, **J**, **va**, **va'**, **k**, **t**] transforms the coefficients

$h$  into  $va'$  under the  $k$ 'th transformation  $U_k$  corresponding to the  $M_k$  matrix. Under this transformation the original

Floquet operator  $H - p_t =$

$va^T h - p_t$  is transformed into  $H' - p_t =$

$$U_k (H - p_t) U_k = va^T M_k h - \alpha_k h_k - p_t =$$

$(va')^T h - p_t$  where  $va'$  is the new set of coefficients.

- **M** :  $n \times n \times n$  tensor containing the transformation matrices,
- **J** :  $n \times n$  matrix,  $h' = Jh$  is a new representation of the  $\mathcal{L}_n$ ,
- **va** : dimension  $n$  list  $va = \{a_1, a_2, \dots, a_n\}$  containing the coefficients of the original Floquet operator,

- **$\mathbf{v}\alpha$**  : dimension  $n$  list  $\mathbf{v}\alpha = \{\alpha_1, \alpha_2, \dots, \alpha_n\}$  containing the transformation parameters for the  $U_A$  transformation,
- **$\mathbf{k}$**  : integer that tags the number of transformation to be used,
- **$\mathbf{t}$**  : time parameter.

```
In[3]:= LieTrans[M_, J_, va_, vα_, k_, t_] :=
      va.M[[k]] - D[vα[[k]], t] J[[k]]
```

## LieGetu

**LieGetu[M, J, va, vα, t]** transforms the original coefficients  $\mathbf{v}\mathbf{a}$  into  $\mathbf{u}$  under the complete transformation  $U_A$  corresponding to  $M_\alpha = M_1 M_2 \dots M_n$ . Under this transformation the original Floquet operator  $H - p_t = \mathbf{v}\mathbf{a} \cdot \mathbf{h} - p_t$  is transformed into  $H' - p_t = U_A (H - p_t) U_A = \mathbf{v}\mathbf{a}^T M_\alpha \mathbf{h} - \dot{\alpha}^T \mathbf{v}^T \mathbf{h}_k - p_t = \mathbf{u}^T \mathbf{h} - p_t$ .

- **$\mathbf{M}$**  : is an  $n \times n \times n$  tensor containing the transformation matrices,
- **$\mathbf{J}$**  :  $n \times n$  matrix,  $\mathbf{h}' = \mathbf{J}\mathbf{h}$  is a new representation of the  $\mathcal{L}_n$ ,
- **$\mathbf{v}\mathbf{a}$**  : dimension  $n$  list  $\mathbf{v}\mathbf{a} = \{a_1, a_2, \dots, a_n\}$  containing the coefficients of the original Floquet operator,
- **$\mathbf{v}\alpha$**  : dimension  $n$  list containing the transformation parameters for the  $U_A$  transformation. The  $\alpha$  parameters must be functions of the time parameter  $t$ .
- **$\mathbf{t}$**  : time parameter.

```

In[4]:= LieGetu[M_, J_, va_, vα_, t_] := Module[{k, vu, vw},
  k = Dimensions[vα][[1]];
  vu = va;
  Do[
    vw = LieTrans[M, J, vu, vα, k1, t];
    vu = vw;
    , {k1, 1, k}];
  vu
]

```

## LieGetDifEqLambda

**LieGetDifEqLambda[J,vi,vα,vβ,λ,ci]** calculates a list containing the differential equations with respect to the auxiliary parameter  $\lambda$  that connects the  $\alpha$  and  $\beta$  parameters.

- **J** :  $n \times n$  matrix,  $h' = J.h$  is a new representation of the  $\mathcal{L}_n$ ,
- **vi** : inverse of the  $n \times n$  matrix  $v$  calculated with `LieGetNu[M,J]`,
- **vα** : dimension  $n$  list  $v\alpha = \{\alpha_1, \alpha_2, \dots, \alpha_n\}$  containing the transformation parameters for the  $U_A$ . The  $\alpha$  parameters must be functions of the auxiliary parameter  $\lambda$ ,
- **vβ** : dimension  $n$  list  $v\beta = \{\beta_1, \beta_2, \dots, \beta_n\}$  containing the transformation parameters for the  $U_B$ . The  $\beta$  parameters are NOT functions of the auxiliary parameter  $\lambda$ ,
- **λ** : is the auxiliary parameter that helps relate the  $\alpha$  and  $\beta$  transformation parameters.

**ci** : is a Boolean variable. If  $ci == \text{True}$ ,  
the initial conditions  $\alpha_1[0] == 0$ ,  $\alpha_2[0] == 0$ , ...,  
 $\alpha_n[0] == 0$  is appended to the list of differential equations. If on  $ci == \text{False}$  then the output is just the list of differential equations,

- **$\lambda$**  : is the auxiliary parameter that helps relate the  $\alpha$  and  $\beta$  transformation parameters.

```
In[5]:= LieGetDifEqLambda[J_, v i_, v α_, v β_, λ_, ci_] :=
Module[{dim, v},
  dim = Dimensions[v α][[1]];
  v = v i. v β;
  If[ci == True,
    Join[Table[D[v α[[k1]], λ] == v[[k1]], {k1, 1, dim}],
      Table[(v α[[k1]] /. λ → 0) == 0, {k1, 1, dim}]],
    Table[D[v α[[k1]], λ] == v[[k1]], {k1, 1, dim}]
  ]
]
```

---

## Main Program

### Definition of the structure constants $c_{i,j,k}$

The elements of this algebra are given by the operators  $h_1 = x^2$ ,  
 $h_2 = x p + p x$ ,  $h_3 = p^2$ . The following lines define the algebra  
dimension and the structure constants.

```

In[6]:= n = 3;
d = Table[0, {k1, 1, n}, {k2, 1, n}, {k3, 1, n}];
d[[1, 2, 3]] = 2;
d[[2, 1, 3]] = -2;
d[[1, 3, 1]] = 4;
d[[3, 1, 1]] = -4;
d[[2, 3, 2]] = -4;
d[[3, 2, 2]] = 4;
R = {{1, 0, 0}, {0, 0, 1}, {0, 1, 0}};
Ri = Inverse[R];
c =
  Table[Sum[R[[k1, m1]] R[[k2, m2]] Ri[[m3, k3]]
    d[[m1, m2, m3]], {m1, 1, n}, {m2, 1, n},
    {m3, 1, n}], {k1, 1, n}, {k2, 1, n}, {k3, 1, n}];

```

Since  $J=\mathcal{I}$ , the structure of the algebra elements is preserved.

```

In[17]:= J = IdentityMatrix[n];

```

## Derivation of the time differential equations for $\alpha_i(t)$

We calculate  $\nu$  using Eq. (12). Notice that in this case  $\nu\alpha = \{\alpha_1(t), \dots, \alpha_n(t)\}$  is a function of time.

```

In[18]:= v $\alpha$  = Table[Subscript[ $\alpha$ , k1][t], {k1, 1, n}];
v $a$  = Table[Subscript[a, k1], {k1, 1, n}];
Ma = LieGetMa[c, J, v $\alpha$ ];
vu = LieGetu[Ma, J, v $a$ , v $\alpha$ , t];
Simplify[vu]

```

$$\begin{aligned}
\text{Out[22]} = & \left\{ e^{4\alpha_2[t]} \left( a_1 - 4a_2\alpha_1[t] + 4a_3\alpha_1[t]^2 - \alpha_1'[t] \right), \right. \\
& a_2 - 2a_3\alpha_1[t] + 2e^{4\alpha_2[t]}\alpha_3[t] \\
& \left( a_1 - 4a_2\alpha_1[t] + 4a_3\alpha_1[t]^2 - \alpha_1'[t] \right) - \alpha_2'[t], e^{-4\alpha_2[t]}a_3 + \\
& 4e^{4\alpha_2[t]}\alpha_3[t]^2 \left( a_1 - 4a_2\alpha_1[t] + 4a_3\alpha_1[t]^2 - \alpha_1'[t] \right) + \\
& \left. 4\alpha_3[t] \left( a_2 - 2a_3\alpha_1[t] - \alpha_2'[t] \right) - \alpha_3'[t] \right\}
\end{aligned}$$

Compare these results with the ones in Eqs. (36)-(38).

The simplified differential equations for  $\alpha_i(t)$  are obtained from Eq. (14)

```

In[23]:= v = LieGetNu[Ma, J];
vi = Inverse[v];
 $\delta$  = Simplify[vi.vu];
MatrixForm[ $\delta$ ]

```

Out[26]//MatrixForm=

$$\begin{pmatrix} a_1 - 4a_2\alpha_1[t] + 4a_3\alpha_1[t]^2 - \alpha_1'[t] \\ a_2 - 2a_3\alpha_1[t] - \alpha_2'[t] \\ e^{-4\alpha_2[t]}a_3 - \alpha_3'[t] \end{pmatrix}$$

Compare these results with the ones in Eqs. (40)-(42).

## Relation between $\alpha(t)$ and $\beta(t)$ via the solution of the $\lambda$ differential equations

Using Eq. (16) we workout the  $\lambda$  differential equations for the  $\alpha_i(\lambda, t)$  parameters. Note that in this case  $v\alpha = \{\alpha_1(\lambda), \dots, \alpha_n(\lambda)\}$  is a function of  $\lambda$  therefore,  $M_a$  and  $v$  have to be recalculated. In



**LieGetDifEqLamda** the condition **ci** is set to **False** in order to avoid setting the initial conditions.

```
In[27]:= vα = Table[Subscript[α, k1][λ], {k1, 1, n}];
Ma = LieGetMa[c, J, vα];
v = LieGetNu[Ma, J];
vi = Inverse[v];
vβ = Table[Subscript[β, k1], {k1, 1, n}];
difeqsλ =
  Simplify[
    ExpToTrig[LieGetDifEqLambda[J, vi, vα, vβ, λ,
      False]]];
MatrixForm[difeqsλ]
```

Out[33]//MatrixForm=

$$\begin{pmatrix} (\cosh[4 \alpha_2[\lambda]] - \sinh[4 \alpha_2[\lambda]]) \beta_1 = \alpha_1'[\lambda] \\ \beta_2 = 2 \beta_1 \alpha_3[\lambda] + \alpha_2'[\lambda] \\ \beta_3 + 4 \beta_1 \alpha_3[\lambda]^2 = 4 \beta_2 \alpha_3[\lambda] + \alpha_3'[\lambda] \end{pmatrix}$$

Compare these results with Eqs. (26)-(28).

These equations are simple enough that we can attempt to solve them with **DSolve**, however, as mentioned above it is easier to solve the system without initial conditions.

```
In[34]:= sol = Simplify[DSolve[difeqsλ, vα, λ][[1]]]
```

$$\text{Out[34]} = \left\{ \begin{aligned} \alpha_3[\lambda] &\rightarrow \frac{\beta_2 + \sqrt{-\beta_2^2 + \beta_1 \beta_3} \tan\left[2(\lambda + C[1]) \sqrt{-\beta_2^2 + \beta_1 \beta_3}\right]}{2 \beta_1}, \\ \alpha_2[\lambda] &\rightarrow C[2] + \frac{1}{2} \log\left[\cos\left[2(\lambda + C[1]) \sqrt{-\beta_2^2 + \beta_1 \beta_3}\right]\right], \\ \alpha_1[\lambda] &\rightarrow C[3] + \frac{1}{2 \sqrt{-\beta_2^2 + \beta_1 \beta_3}} (\cosh[4 C[2]] - \sinh[4 C[2]]) \\ &\quad \beta_1 \tan\left[2(\lambda + C[1]) \sqrt{-\beta_2^2 + \beta_1 \beta_3}\right] \end{aligned} \right\}$$

Setting  $\lambda=1$  we can obtain a relation between  $\alpha(t)$  and  $\beta(t)$  of the

form (17).

```
In[35]:= va1 = Table[Subscript[α, k1], {k1, 1, n}];
eqs = Table[va1[[k1]] == ((va[[k1]] /. sol) /. {λ → 1}),
{ k1, 1, n}]
```

$$\text{Out[36]} = \left\{ \begin{aligned} \alpha_1 &= C[3] + \frac{1}{2 \sqrt{-\beta_2^2 + \beta_1 \beta_3}} (\text{Cosh}[4 C[2]] - \text{Sinh}[4 C[2]]) \\ &\quad \beta_1 \text{Tan} \left[ 2 (1 + C[1]) \sqrt{-\beta_2^2 + \beta_1 \beta_3} \right], \\ \alpha_2 &= C[2] + \frac{1}{2} \text{Log} \left[ \text{Cos} \left[ 2 (1 + C[1]) \sqrt{-\beta_2^2 + \beta_1 \beta_3} \right] \right], \\ \alpha_3 &= \frac{\beta_2 + \sqrt{-\beta_2^2 + \beta_1 \beta_3} \text{Tan} \left[ 2 (1 + C[1]) \sqrt{-\beta_2^2 + \beta_1 \beta_3} \right]}{2 \beta_1} \end{aligned} \right\}$$

In principle, one could obtain the inverse relations of the form (18), however, it is easier to resort to the eigenvalue one eigenvectors of  $M_a^T$ .

## Relation between $\alpha(t)$ and $\beta(t)$ via the eigenvalue one eigenvectors of $M_a^T$

Working out the inverse relation between  $\alpha$  and  $\beta$  might be difficult in this case given the complexity of the previous equations.

Therefore, it is convenient to obtain a relation between  $\alpha(t)$  and  $\beta(t)$  by obtaining the eigenvalue one eigenvectors of  $M_a^T$ . There is one eigenvalue one eigenvector.

```

In[37]:=  $\mathbf{v}\alpha = \text{Table}[\text{Subscript}[\alpha, \mathbf{k1}], \{\mathbf{k1}, 1, \mathbf{n}\}];$ 
 $\mathbf{Ma} = \text{LieGetMa}[\mathbf{c}, \mathbf{J}, \mathbf{v}\alpha];$ 
 $\mathbf{Mat} = \text{Transpose}[\mathbf{Ma}[[\mathbf{n} + 1]]];$ 
 $\mathbf{eval} = \text{Simplify}[\text{Eigenvalues}[\mathbf{Mat}]];$ 
 $\mathbf{evec} = \text{Simplify}[\text{Eigenvectors}[\mathbf{Mat}]];$ 
 $\mathbf{eval}[[1]]$ 
 $\rho_1 = \text{Simplify}[\mathbf{evec}[[1]]]$ 
 $\beta_1 = \gamma_1 \rho_1$ 

```

Out[42]= 1

Out[43]=  $\left\{ \frac{\alpha_1}{\alpha_3}, \frac{1 - e^{-4\alpha_2} + 4\alpha_1\alpha_3}{4\alpha_3}, 1 \right\}$

Out[44]=  $\left\{ \frac{\alpha_1 \gamma_1}{\alpha_3}, \frac{(1 - e^{-4\alpha_2} + 4\alpha_1\alpha_3) \gamma_1}{4\alpha_3}, \gamma_1 \right\}$

Compare this last result with the one in Eq. (29).
